# Supplementary material for: Mapping polygons to the grid with small Hausdorff and Fr\'echet distance
Source: arXiv:1606.06660 source file (2016-06-21)

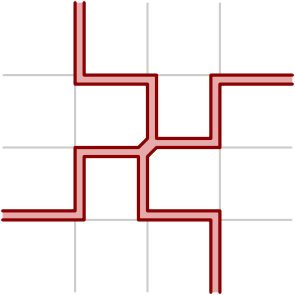

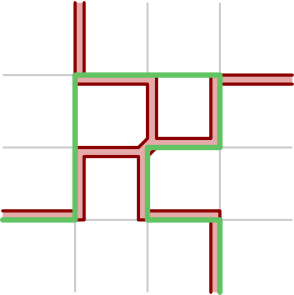

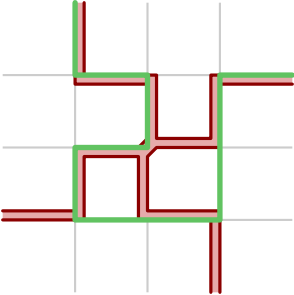

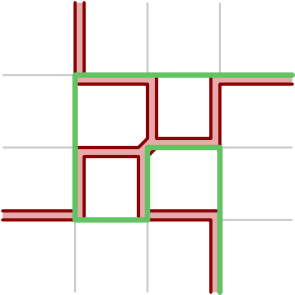

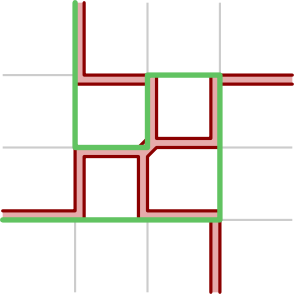

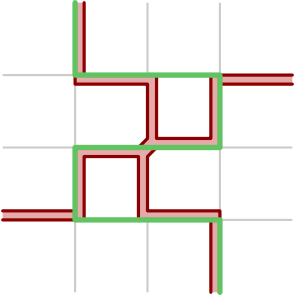

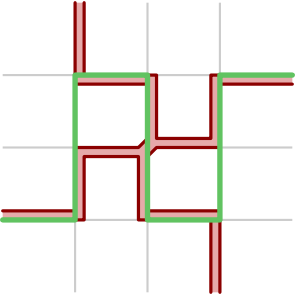

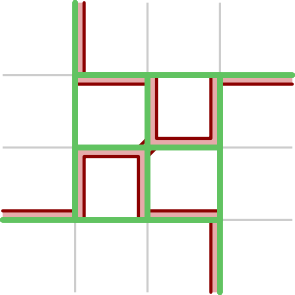

Supplement: Supplementary file 1 [file hausdorff-hard-vertex.pdf]
