# Supplementary material for: Mapping polygons to the grid with small Hausdorff and Fr\'echet distance
Source: arXiv:1606.06660 source file (2016-06-21)

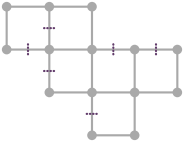

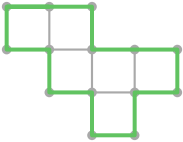





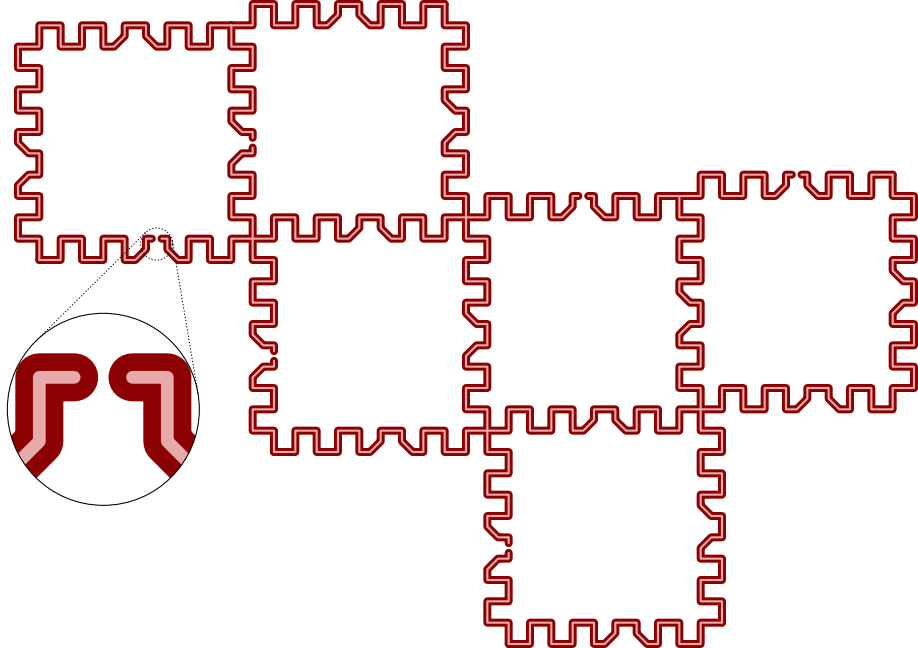

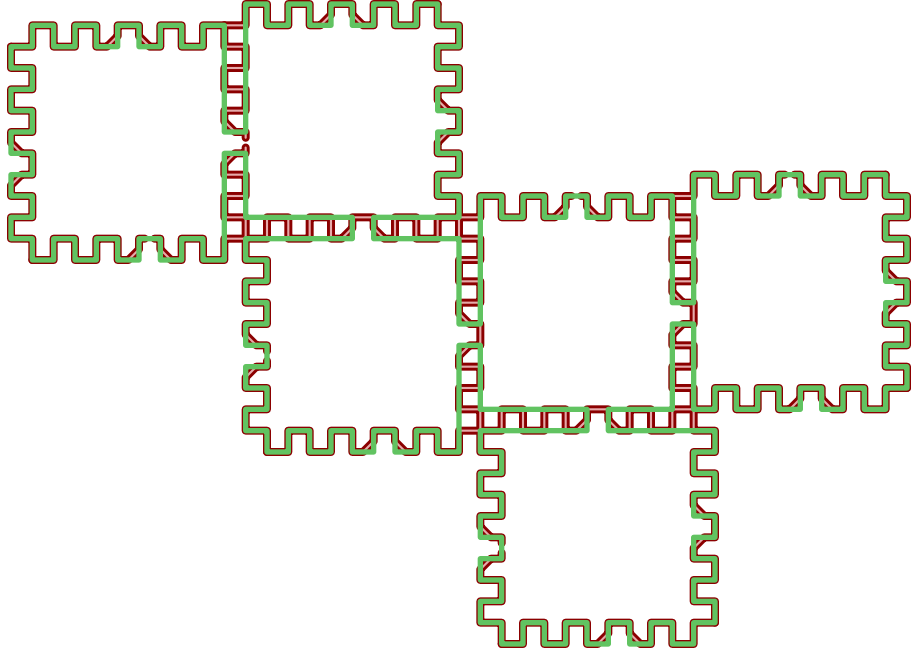

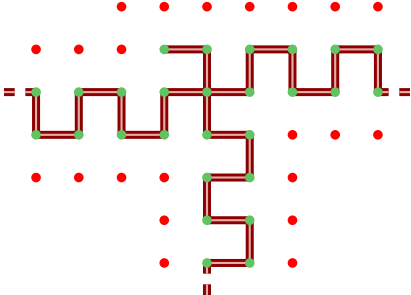

Supplement: Supplementary file 2 [file hausdorff-hard.pdf]
